# Supplementary material for: Addressing Security and Privacy Challenges in Internet of Things
Source: arXiv:1807.06724 source file (2018-07-18)
Supplement: Supplementary file 1 [file implementation.tex]

\chapter{Implementation Details\label{ch:implementation}}

Appendices are just chapters, included after the $\backslash appendix$ command.

\section{Switching Formats}
When switching \texttt{printmode} on and off (see Section~\ref{sec:usage:options}), you may need to delete the output .aux files to get the document code to compile correctly. This is because the hyperref package is switched off for \texttt{printmode}, but this package inserts extra tags into the contents lines in the auxiliary files for PDF links, and these can cause errors when the package is not used.

\section{Long Tables}

Long tables span multiple pages. By default they are treated like body text, but we want them to be single spaced all the time. The class therefore defines a new command, $\backslash tablespacing$, that is placed before a long table to switch to single spacing when the rest of the document is in double spacing mode. Another command, $\backslash bodyspacing$, is placed after the long table to switch back to double spacing. Normal tables using \texttt{tabular} automatically use single spacing and do not require the extra commands.

When the documentclass is defined with the `singlespace' option, these commands are automatically adjusted to stay in single spacing after the long table.

Make sure there is always at least one blank line after the $\backslash bodyspacing$ command before the end of the file.

Some times long tables do not format correctly on the first pass. If the column widths are wrong, try running the \LaTeX compiler one or two extra times to allow it to better calculate the column widths.

If you want your long table to break pages at a specific point, you can insert the command $\backslash pagebreak[4]$, to tell \LaTeX that it really should put a page break there. $\backslash pagebreak[2]$ gives it a hint that this is a good place for a page break, if needed. If there's a row that really should not be broken across a page, use $\backslash \backslash *$, which will usually prevent a pagebreak. 

\section{Booktabs}
The booktabs package is included to print nicer tables. See the package documentation~\cite{fear2005booktabs} for more details and motivation. Generally, all vertical lines are removed from the tables for a better visual appearance (so don't put them in), and better spacing and line thicknesses are used for the horizontal rules. The rules are defined as $\backslash toprule$ at the top of the table, $\backslash midrule$ in between the heading and the body of the table (or between sections of the table), and $\backslash bottomrule$ at the end of the table. $\backslash cmidrule$ can be used with the appropriate options to have a rule that spans only certain columns of the table.

\section{Bibliography and Footnotes}

The bibliography and any footnotes can also be single spaced, even for the electronic copy. The template is already setup to do this.

Bibliography entries go in the .bib file. As usual, be sure to compile the \LaTeX code, then run BibTeX, and then run \LaTeX again.

To cite websites and other electronically accessed materials, you can use the `@electronic' type of BibTeX entry, and use the `howpublished' field to include the URL of the source material.

The formatting of bibliography entries will be done automatically. Usually the titles are changed to have only the first word capitalized. If you'd prefer to have your original formatting preserved, place the title in an extra set of curly braces, i.e., ``title = \{\{My title has an AcroNyM that should stay unchanged\}\},''.

\section{Figures and Tables}
The captions of figures and tables take an optional parameter in square brackets, specifying the caption text to be used in the Table of Contents. The regular caption in curly braces is used for the table itself.

Generally captions for tables are placed above the table, while captions for figures are placed below the figure.
