# Supplementary material for: Addressing Security and Privacy Challenges in Internet of Things
Source: arXiv:1807.06724 source file (2018-07-18)
Supplement: Supplementary file 2 [file printing.tex]

\chapter{Printing and Binding\label{ch:printing}}

\section{Printing}

For the library copies of your dissertation, you must use archival quality printing and binding. This means acid-free paper, containing at least 25\% cotton fiber. Triangle Repocenter on Nassau Street in Princeton offers both 25\% cotton paper and 100\% cotton paper. Most people choose the 25\% cotton paper, and this is generally recommended by the binders. The 100\% copy paper is somewhat thicker and the extra expense is unnecessary. 

Triangle offers online submission of your printing and binding order at: \url{http://triangleprinceton.com/collegiatebinding/thesis/}. If you request binding from them, they will deliver the paper copies to Smith-Shattuck Bookbinding for you and allow you to pick up the completed copies at their store on Nassau Street. The whole process takes 2-3 business days, but check with them in advance during the busy thesis-printing season in April and May. 

Currently, your printed and bound dissertation copies can be single spaced. Only the electronic copy submitted to ProQuest must be double spaced. All copies must be printed single-sided, with specific margins. 

\section{Binding}

An archival-quality sewn binding is required for the library copies of your dissertation. Smith-Shattuck Bookbinding is highly recommended, and is used by most students. Triangle Repocenter will send your copies there for you, greatly simplifying the process, but you can call Smith-Shattuck with special requests. 

The ``library standard'' sewn binding is sufficient for the copies to be sent to Mudd Library. It uses a black buckram cloth cover, which is the most popular option. For extra copies for yourself and your family members, you can choose ``buckram roundback binding'', which adds decorative lines on the spine, and printing of the title and author on the front cover. For a small additional fee, you can include the Princeton University shield on the front cover and a ribbon bookmark. Leather covers are also available. See Smith-Shattuck's website for more details at: \url{http://www.thesisbookbinding.com/}.
